# Supplementary material for: Monocular Depth Estimation for Soft Visuotactile Sensors
Source: arXiv:2101.01677 source file (2021-01-05)
Supplement: Supplementary file 1 [file supp_networks.tex]

An architectural overview of each depth network considered in this work can be found in Table \ref{tab:networks} (for a more detailed description please refer to~\
\cite{he2016deep,packnet,lee2019big}). Each network receives as input a $224 \times 224$ grayscale image, and outputs a $224 \times 224$ image with per-pixel metric depth estimates.  We also include inference times for each network (batch size of $1$, measured on a Titan V100 GPU card), with \textit{ResNet} achieving the fastest performance, with 58 fps (frames per second); followed by \textit{PackNet}, with 24 fps; and finally \textit{BTS}, with 20 fps. Additionally, we show a high level diagram of the proposed learning framework in Figure~\ref{fig:framework}.

\begin{figure}[h!]
\vspace{5mm}
\includegraphics[width=\linewidth]{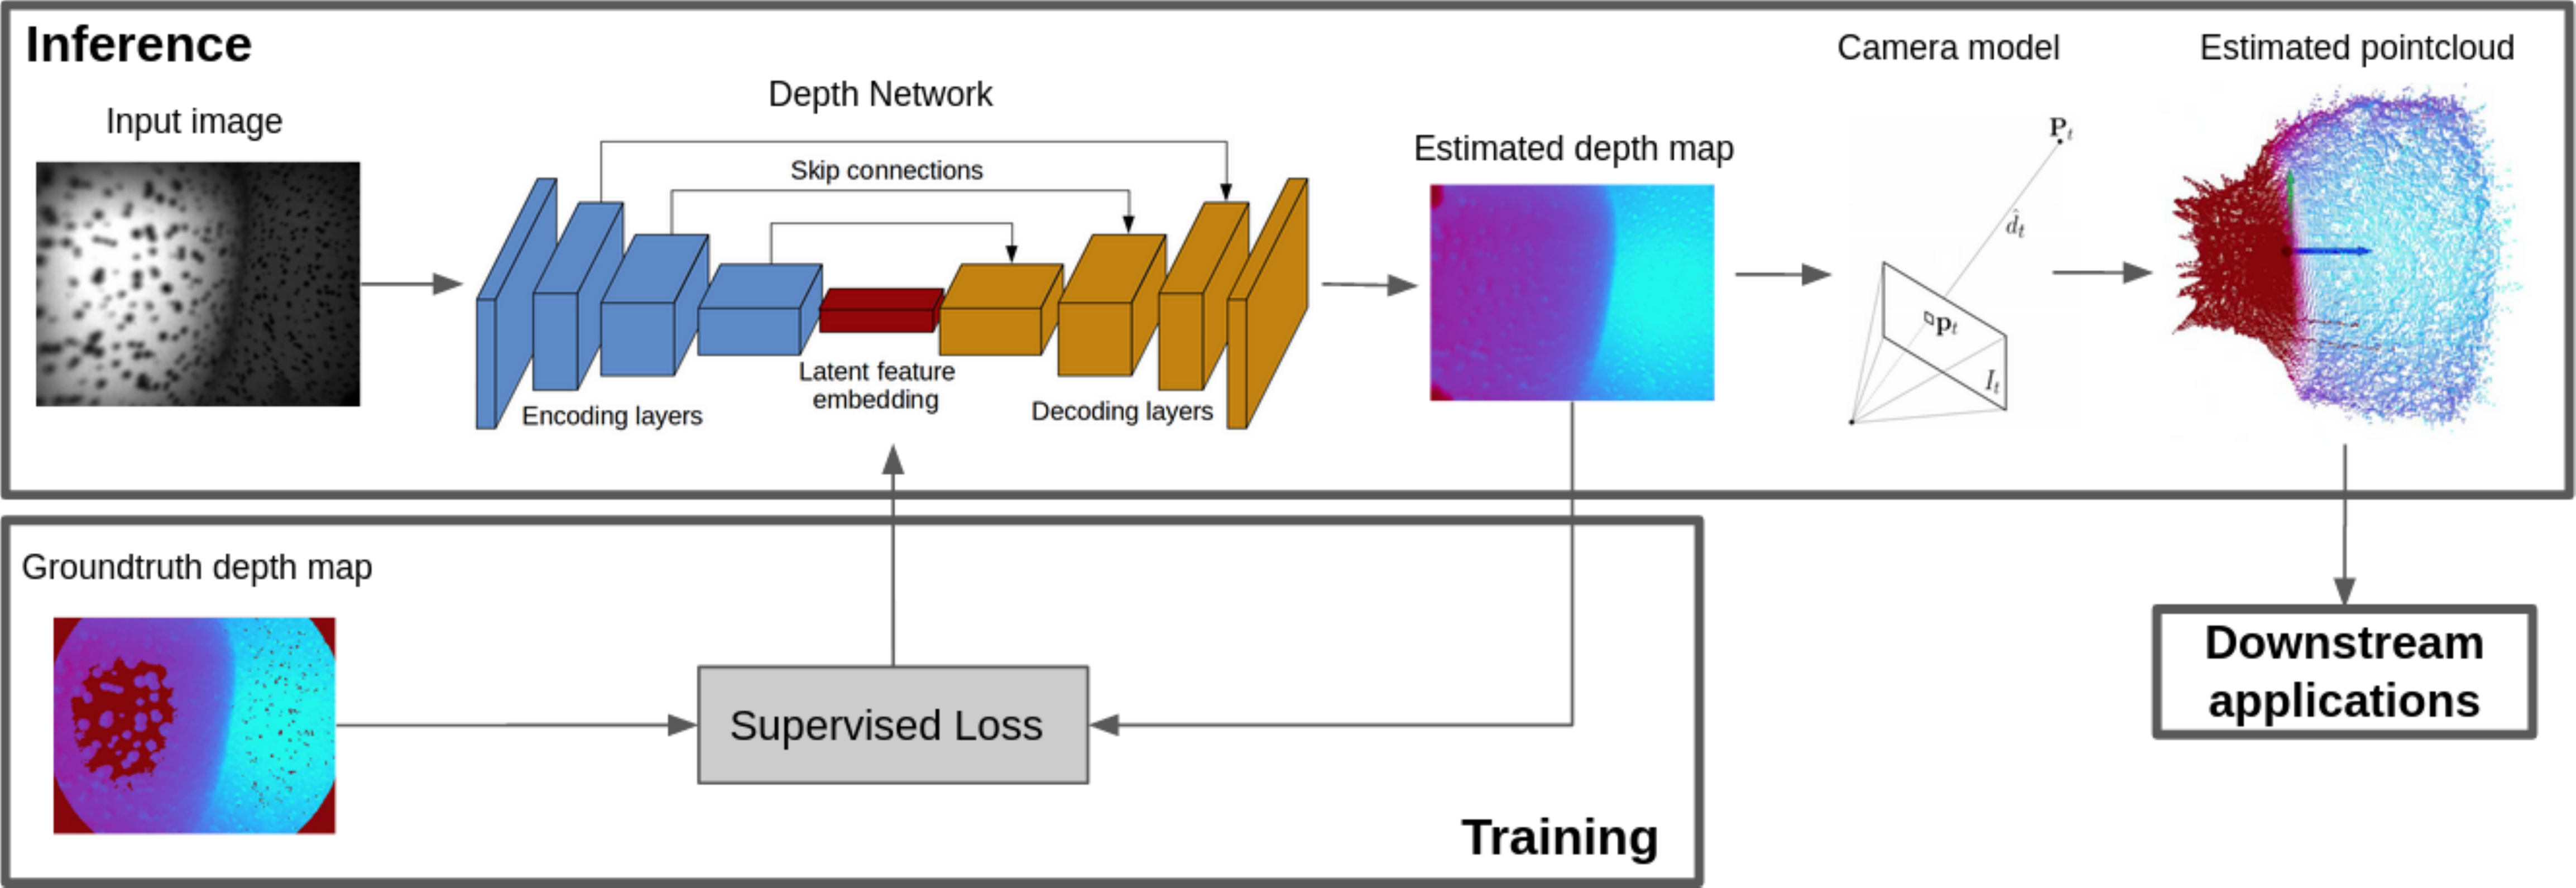}
\caption{Diagram of our proposed framework. We use as input a $H \times W$ grayscale image, that is processed by our \textit{Depth Network} to produce an estimated depth map of the same resolution. At training time, the corresponding ground-truth depth map is also provided, and the \textit{Depth Network} is optimized as to minimize the difference between estimated and ground-truth depth maps, given an objective function (Equation 2, main paper). The estimated depth map is lifted to 3D using the camera model, to produce an estimated pointcloud, and can then be used for downstream applications (e.g. pose estimation).}
\label{fig:framework}
\end{figure}

\begin{table*}[!t]%
\small
  \centering
\resizebox{0.49\linewidth}{!}{
\subfloat[ResNet \cite{godard2018digging2} (58  fps)]{
%%%%%%%%%%%%%%%%%%%%%%%%%%%%%%%%%%%%%%%%%%%%%%%%%%%
\begin{tabular}[b]{l|l|c|c|c}
\toprule
& \textbf{Layer Description} & \textbf{K} & \textbf{S} & \textbf{Out. Dim.} \\ 
\toprule
\multicolumn{5}{c}{\textbf{ResidualBlock (K, S)}} \\ 
\midrule
\#A & Conv2d$\shortrightarrow$BN$\shortrightarrow$ReLU & K & 1 &  \\
\#B & Conv2d$\shortrightarrow$BN$\shortrightarrow$ReLU & K & S &  \\
\toprule
\multicolumn{5}{c}{\textbf{UpsampleBlock (\#skip)}} \\ 
\midrule
\#C & Conv2d$\shortrightarrow$BN$\shortrightarrow$ReLU$\shortrightarrow$Upsample    & 3 & 1 & \\
\#D & Conv2d ($\#C\oplus\#skip$)$\shortrightarrow$BN$\shortrightarrow$ReLU          & 3 & 1 & \\
\toprule
\toprule
\#0 & Input RGB image & - & - & 3$\times$H$\times$W \\ 
\midrule
\multicolumn{5}{c}{\textbf{Encoder}} \\ \hline
\#1  & Conv2d$\shortrightarrow$BN$\shortrightarrow$ReLU   & 7 & 1 &  64$\times$H$\times$W \\
\#2  & Max. Pooling                                       & 3 & 2 &  64$\times$H/2$\times$W/2 \\
\#3  & ResidualBlock (x2)                                 & 3 & 2 &  64$\times$H/4$\times$W/4 \\
\#4  & ResidualBlock (x2)                                 & 3 & 2 & 128$\times$H/8$\times$W/8 \\
\#5  & ResidualBlock (x2)                                 & 3 & 2 & 256$\times$H/16$\times$W/16 \\
\#6  & ResidualBlock (x2)                                 & 3 & 2 & 512$\times$H/32$\times$W/32 \\
\midrule
\multicolumn{5}{c}{\textbf{Depth Decoder}} \\ 
\midrule
\#7 & UpsampleBlock (\#5)    & 3 & 1 & 256$\times$H/16$\times$W/16 \\
\#8 & UpsampleBlock (\#4)    & 3 & 1 & 128$\times$H/8$\times$W/8 \\
\#9 & UpsampleBlock (\#3)    & 3 & 1 & 64$\times$H/4$\times$W/4 \\
\#10 & UpsampleBlock (\#2)   & 3 & 1 & 32$\times$H/2$\times$W/2 \\
\#11 & UpsampleBlock (\#1)   & 3 & 1 & 32$\times$H$\times$W \\
\#12 & Conv2d$\shortrightarrow$Sigmoid  & 3 & 1 & 1$\times$H$\times$W \\
\bottomrule
\end{tabular}
}}
%%%%%%%%%%%%%%%%%%%%%%%%%%%%%%%%%%%%%%%%%%%%%%%%%%%
\resizebox{0.49\linewidth}{!}{
\subfloat[PackNet \cite{packnet} (24 fps)]{
\begin{tabular}[b]{l|l|c|c|c}
\toprule
 & \textbf{Layer Description} & \textbf{K} & \textbf{S} & \textbf{Out. Dim.} \\ 
\midrule
\multicolumn{5}{c}{\textbf{ResidualBlock (K, S)}} \\ \hline
\#A & Conv2d$\shortrightarrow$GN$\shortrightarrow$ELU & K & 1 &  \\
\#B & Conv2d$\shortrightarrow$GN$\shortrightarrow$ELU & K & 1 &  \\
\#C & Conv2d$\shortrightarrow$GN$\shortrightarrow$ELU$\shortrightarrow$Dropout & K & S &  \\
\toprule
\multicolumn{5}{c}{\textbf{UpsampleBlock (\#skip)}} \\ \hline
\#D & Unpacking         & 3 & 1 & \\
\#E & Conv2d ($\#D\oplus\#skip$)$\shortrightarrow$GN$\shortrightarrow$ELU    & 3 & 1 & \\
\toprule
\toprule
\#0 & Input RGB image & - & - & 3$\times$H$\times$W \\ 
\midrule
\multicolumn{5}{c}{\textbf{Encoder}} \\ \hline
\#1 & Conv2d$\shortrightarrow$GN$\shortrightarrow$ELU & 5 & 1 & 64$\times$H$\times$W \\
\#2 & Conv2d$\shortrightarrow$GN$\shortrightarrow$ELU$\shortrightarrow$Packing & 7 & 1 & 64$\times$H$\times$W \\
\#3 & ResidualBlock (x2)$\shortrightarrow$Packing & 3 & 1 & 64$\times$H/4$\times$W/4 \\
\#4 & ResidualBlock (x2)$\shortrightarrow$Packing & 3 & 1 & 128$\times$H/8$\times$W/8 \\
\#5 & ResidualBlock (x3)$\shortrightarrow$Packing & 3 & 1 & 256$\times$H/16$\times$W/16 \\
\#6 & ResidualBlock (x3)$\shortrightarrow$Packing & 3 & 1 & 512$\times$H/32$\times$W/32 \\
\midrule
\multicolumn{5}{c}{\textbf{Depth Decoder}} \\ \hline
\#7  & UpsampleBlock (\#5) & 3 & 1  & 512$\times$H/16$\times$W/16 \\
\#8  & UpsampleBlock (\#4) & 3 & 1  & 256$\times$H/8$\times$W/8 \\
\#9  & UpsampleBlock (\#3) & 3 & 1  & 128$\times$H/4$\times$W/4 \\
\#10  & UpsampleBlock (\#2) & 3 & 1  & 64$\times$H/2$\times$W/2 \\
\#11  & UpsampleBlock (\#1) & 3 & 1  & 64$\times$H$\times$W \\
\#12 & Conv2d $\shortrightarrow$ Sigmoid & 3 & 1 &   1$\times$H$\times$W \\
\bottomrule
\end{tabular}
}}
%%%%%%%%%%%%%%%%%%%%%%%%%%%%%%%%%%%%%%%%%%%%%%%%%%%
\resizebox{0.50\linewidth}{!}{
\subfloat[BTS \cite{lee2019big} (20 fps)]{
\begin{tabular}[b]{l|l|c|c|c}
\toprule
& \textbf{Layer Description} & \textbf{K} & \textbf{S} & \textbf{Out. Dim.} \\ 
\toprule
\multicolumn{5}{c}{\textbf{ResidualBlock (K, S)}} \\ 
\midrule
\#A & Conv2d$\shortrightarrow$BN$\shortrightarrow$ReLU & 1 & 1 &  \\
\#B & Conv2d$\shortrightarrow$BN$\shortrightarrow$ReLU & K & 1 &  \\
\#C & Conv2d$\shortrightarrow$BN$\shortrightarrow$ReLU & 1 & S &  \\
\toprule
\multicolumn{5}{c}{\textbf{UpsampleBlock}} \\ 
\midrule
\#D & UpsampleBlock (2x) & & &\\ 
\#E & Conv2d$\shortrightarrow$BN$\shortrightarrow$ReLU  & 3 & 1 & \\
\toprule
\multicolumn{5}{c}{\textbf{Conv2dBlock}} \\ 
\midrule
\#F & Conv2d$\shortrightarrow$BN$\shortrightarrow$ReLU & 3 & 1 &  \\
\#G & Conv2d$\shortrightarrow$BN$\shortrightarrow$ReLU & 1 & 1 &  \\
\toprule
\toprule
\#0 & Input RGB image & - & - & 3$\times$H$\times$W \\ 
\midrule
\multicolumn{5}{c}{\textbf{Encoder}} \\ \hline
\#1  & Conv2d$\shortrightarrow$BN$\shortrightarrow$ReLU   & 7 & 2 &  64$\times$H/2$\times$W/2 \\
\#2  & Max. Pooling                 & 3 & 2 &   64$\times$H/2$\times$W/2 \\
\#3  & ResidualBlock (x3)           & 3 & 2 &  256$\times$H/4$\times$W/4 \\
\#4  & ResidualBlock (x4)           & 3 & 2 &  512$\times$H/8$\times$W/8 \\
\midrule
\multicolumn{5}{c}{\textbf{Depth Decoder}} \\ 
\midrule
\#5  & ASPP (\#4)                                   & 3 & 1 & 512$\times$H/8$\times$W/8 \\
\#6  & Local Planar Guidance (\#5)                  & 3 & 1 & 512$\times$H$\times$W \\
\#7  & UpsampleBlock (\#5)                          & 3 & 1 & 256$\times$H/4$\times$W/4 \\
\#8  & Downsample (\#6)                             & 3 & 1 & 256$\times$H/4$\times$W/4 \\
\#9  & Conv2dBlock (\#3$\oplus$\#7$\oplus$\#8)  & 3 & 1 & 256$\times$H/4$\times$W/4 \\
\#10 & Local Planar Guidance (\#9)                  & 3 & 1 & 256$\times$H$\times$W \\
\#11 & UpsampleBlock (\#9)                          & 3 & 1 & 128$\times$H/2$\times$W/2 \\
\#12 & Downsample (\#10)                            & 3 & 1 & 128$\times$H/2$\times$W/2 \\
\#13 & Conv2dBlock (\#2$\oplus$\#11$\oplus$\#12)    & 3 & 1 & 128$\times$H/2$\times$W/2 \\
\#14 & Local Planar Guidance (\#15)                 & 3 & 1 & 128$\times$H$\times$W \\
\#15 & UpsampleBlock (\#16)                         & 3 & 1 &  64$\times$H$\times$W \\
\#16 & Reduction (\#17)                             & 3 & 1 &  32$\times$H$\times$W \\
\#17 & Conv2dBlock (\#6$\oplus$\#10$\oplus$\#14$\oplus$\#16) & 3 & 1 & 1$\times$H$\times$W \\
\#18 & Sigmoid (\#17) & & & 1$\times$H$\times$W \\
\bottomrule
\end{tabular}
}}
\\
%%%%%%%%%%%%%%%%%%%%%%%%%%%%%%%%%%%%%%%%%%%%%%%%%%%
\caption{
\textbf{Different depth networks used in this work.} The depth network outputs $1 \times H \times W$ tensors with predicted inverse depth values, that are scaled between the minimum and maximum depth ranges. \emph{BN} stands for Batch Normalization \cite{ioffe2015batch}, \emph{GN} for Group Normalization \cite{WuH18}, \emph{Dropout} is described in \cite{dropout14}, \emph{Upsample} doubles spatial dimensions using bilinear interpolation, \emph{ReLU} are Rectified Linear Units and \emph{ELU} are Exponential Linear Units \cite{clevert2016fast}. The symbol $\oplus$ indicates feature concatenation. Inference times were calculated using a Titan V100 GPU and batch size of $1$.
}
%%%%%%%%%%%%%%%%%%%%%%%%%%%%%%%%%%%%%%%%%%%%%%%%%%%
\label{tab:networks}
\end{table*}

% \begin{tabularx}{0.5\textwidth}{X|l}
% \shortrightarrowprule
% asdfasdf
% \shortrightarrowprule
% \end{tabularx}
