# Supplementary material for: Monocular Depth Estimation for Soft Visuotactile Sensors
Source: arXiv:2101.01677 source file (2021-01-05)
Supplement: Supplementary file 2 [file supp_resnet.tex]

\begin{table}[!h]
\small

\centering
% \resizebox{\linewidth}{!}{
\begin{tabular}{l|l|c|c}
\toprule
& \textbf{Layer Description} & \textbf{K} & \textbf{Output Tensor Dim.} \\ 
\toprule
\#0 & Input RGB image & & 3$\times$H$\times$W \\ 
\midrule
\midrule
\multicolumn{4}{c}{\textbf{ResidualBlock}} \\ \hline
& Conv2d + BatchNorm + ReLU & 3 &  \\
& Conv2d + BatchNorm        & 3 &  \\
\midrule
\multicolumn{4}{c}{\textbf{Depth Encoder}} \\ \hline
\#1  & Conv2d (S2) + BatchNorm + ReLU & 7 &  64$\times$H/2$\times$W/2 \\
\#2  & Conv2d + BatchNorm + ReLU            & 3 &  64$\times$H/2$\times$W/2 \\
\#3  & ResidualBlock (\#2)  x2              & - &  64$\times$H/2$\times$W/2 \\
\#4  & Max. Pooling ($\times$1/2)          & 3 &  64$\times$H/4$\times$W/4 \\
\#5  & ResidualBlock (\#3 + \$2) x2         & - & 128$\times$H/4$\times$W/4 \\
\#6  & Max. Pooling ($\times$1/2)          & 3 & 128$\times$H/8$\times$W/8 \\
\#7  & ResidualBlock (\#4 + \#3) x2         & - & 256$\times$H/8$\times$W/8 \\
\#8  & Max. Pooling ($\times$1/2)          & 3 & 256$\times$H/16$\times$W/16 \\
\#9  & ResidualBlock (\#5 + \#4) x2         & - & 512$\times$H/16$\times$W/16 \\
\midrule
\multicolumn{4}{c}{\textbf{Depth Decoder}} \\ 
\midrule
\#10 & Conv2D + ELU (\#9)                                   & 3 & 128$\times$H/16$\times$W/16 \\
\#11 & Conv2D + Upsample (\#10)                             & 3 & 128$\times$H/8$\times$W/8  \\
\textbf{\#12} & Conv2D + Sigmoid                            & 3 & 1$\times$H/8$\times$W/8 \\
\#13 & Conv2D + ELU                                         & 3 & 64$\times$H/8$\times$W/8 \\
\#14 & Conv2D + Upsample(\#7 $\oplus$ \#13)                 & 3 & 64$\times$H/4$\times$W/4  \\
\textbf{\#15} & Conv2D + Sigmoid                            & 3 & 1$\times$H/8$\times$W/8 \\
\#16 & Conv2D + ELU                                         & 3 & 32$\times$H/4$\times$W/4 \\
\#17 & Conv2D + Upsample (\#5 $\oplus$ \#16)                & 3 & 32$\times$H/2$\times$W/2  \\
\textbf{\#18} & Conv2D + Sigmoid                            & 3 & 1$\times$H/8$\times$W/8 \\
\#19 & Conv2D + ELU                                         & 3 & 16$\times$H/2$\times$W/2 \\
\#20 & Conv2D + Upsample (\#3 $\oplus$ \#19)                & 3 & 16$\times$H$\times$W  \\
\textbf{\#21} & Conv2D + Sigmoid                            & 3 & 1$\times$H$\times$W \\
\bottomrule
\end{tabular}
% }
\caption{\textbf{ResNet architecture.} Line numbers in bold indicate output inverse depth layer scales. \emph{Upsample} is a nearest-neighbor interpolation operation that doubles the spatial dimensions of the input tensor. $\oplus$ denotes feature concatenation for skip connections.}
\label{table:supp-resnet-arch}
\end{table}
